# Supplementary material for: Weak 21st-century AMOC response to Greenland meltwater in a strongly eddying ocean model
Source: arXiv:2602.17235 ancillary file (2026-05-23)
Supplement: Supplementary file 1 [file Supplement_MD26.pdf]

# Supporting Information for "Weak 21st-century AMOC response to Greenland meltwater in a strongly eddying ocean model"

O. Mehling and H. A. Dijkstra

Institute for Marine and Atmospheric Science, Utrecht University, Utrecht, The Netherlands

**Contents of this file**

1. Text S1 and S2
2. Table S1
3. Figures S1 to S5

**Text S1: Derivation of ocean model forcing from CMIP6**

POP in ocean-only mode is forced with a total of 11 seasonally and spatially resolved fields representing wind stress, surface freshwater, and surface heat flux forcing (Table S1), which were previously derived from the CORE-II "normal-year" forcing product (Large & Yeager, 2004) based on the 1958–2000 climatology of the NCEP/NCAR reanalysis.

Following the strategy of Li, England, Hogg, Rintoul, and Morrison (2023), the time-varying ocean model forcing for the historical + SSP5-8.5 simulations was derived from the CMIP6 multi-model mean as follows. First, we identified the CMIP6 variables matching the POP forcing variables (Table S1) and obtained these fields for the period 1958–2100 for all CMIP6 models available via the Google Cloud Storage of the Pangeo/ESGF Cloud Data Working Group. For each model and each variable, the monthly climatology of the reference period 1958–2000 was subtracted to obtain anomalies. Then, all fields were regridded to a regular 1°x1° grid before taking the mean across all CMIP6 models, thereby

obtaining the CMIP6 multi-model mean anomaly. This approach improves upon the method of Li et al. (2023), who only prescribed zonal mean (instead of 2D-resolved) anomalies. To isolate long-term changes and for consistency with the control run, which does not feature any forced interannual variability, all forcing anomalies were subsequently smoothed with a 20-year running mean. Finally, they were regridded bilinearly to the native ocean grid of POP and added to the original "normal-year" forcing fields to obtain a time-dependent historical + SSP5-8.5 forcing product.

This procedure could be successfully applied to 9 of the 11 forcing variables – all except river runoff and the prescribed sea-ice concentration. River runoff in CMIP6 is only consistently available on the land grid, which would require the application of a river routing scheme on each model's native grid. Because it has been shown that runoff only contributes marginally to Atlantic freshwater budget changes under future warming (Jüling et al., 2021), we therefore decided to keep river runoff constant. In any case, the global warming-induced background AMOC weakening is mostly driven by heat flux and not freshwater flux anomalies (Todd et al., 2020; Couldrey et al., 2023), as we also verified in LR-POP (not shown).

Due to the skewed distributions and large mean-state model biases in sea-ice cover, a different approach was taken for the prescribed sea-ice concentrations. First, a bias correction was applied to the sea ice concentration fields of each model following the "multiplicative correction" method from Sec. 3.2 of Melia, Haines, and Hawkins (2015). Second, for each month, the multi-model median (of the fields themselves, not their anomalies) was taken. The combination of both approaches assured a reasonable match with the observed present-day sea ice state and physically consistent sea ice concentration fields throughout the SSP5-8.5 scenario.

**Text S2: Greenland meltwater forcing**

The time-dependent Greenland meltwater forcing for the "Meltwater" simulations is derived from an existing historical + SSP5-8.5 simulation with a fully coupled climate–ice sheet model, the Community Earth System Model (CESM2) coupled to the Community Ice Sheet Model (CISM2) (Muntjewerf et al., 2020, 2021). This model used a nominal 1° resolution for the climate model and around 5 km resolution for the Greenland ice sheet model. For consistency with the ocean model forcing in HR-POP, Greenland runoff forcing is derived as an anomaly with respect to the 1958–2000 period. This is a reasonable approach since HR-POP does have some (time-constant) runoff of the order of 9 mSv inserted at coastal grid points in the "normal-year" forcing run, which is in good agreement with observational estimates of Greenland runoff during that period (Bamber et al., 2018).

The ice sheet runoff is aggregated into the seven standard drainage basins (Mouginot et al., 2019) and inserted into the ocean in regions within about 30 km of the coast in HR-POP (Fig. S1b). The resulting input time series by region are shown in Fig. S1a. The seasonal cycle of runoff is retained but the interannual variability is smoothed out with a 20-year running mean, similar to the smoothing applied to all other forcing variables.

## References

Bamber, J. L., Tedstone, A. J., King, M. D., Howat, I. M., Enderlin, E. M., van den Broeke, M. R., & Noel, B. (2018). Land Ice Freshwater Budget of the Arctic and North Atlantic Oceans: 1. Data, Methods, and Results. *J. Geophys. Res. Oceans*, *123*, 1827–1837. doi: 10.1002/2017JC013605

Couldrey, M. P., Gregory, J. M., Dong, X., Garuba, O., Haak, H., Hu, A., … Zanna, L. (2023, April). Greenhouse-gas forced changes in the Atlantic meridional overturning circulation and related worldwide sea-level change. *Clim. Dyn.*, *60*, 2003–2039. doi: 10.1007/s00382-022-06386-y

Jüling, A., Zhang, X., Castellana, D., von der Heydt, A. S., & Dijkstra, H. A. (2021, May). The Atlantic's freshwater budget under climate change in the Community Earth System Model with strongly eddying oceans. *Ocean Sci.*, *17*, 729–754. doi: 10.5194/os-17-729-2021

Large, W. G., & Yeager, S. G. (2004, May). *Diurnal to Decadal Global Forcing For Ocean and Sea-Ice Models: The Data Sets and Flux Climatologies* (NCAR Technical Note). Boulder, Colorado: National Center for Atmospheric Research.

Li, Q., England, M. H., Hogg, A. M., Rintoul, S. R., & Morrison, A. K. (2023, March). Abyssal ocean overturning slowdown and warming driven by Antarctic meltwater. *Nature*, *615*, 841–847. doi: 10.1038/s41586-023-05762-w

Melia, N., Haines, K., & Hawkins, E. (2015, December). Improved Arctic sea ice thickness projections using bias-corrected CMIP5 simulations. *The Cryosphere*, *9*, 2237–2251. doi: 10.5194/tc-9-2237-2015

Mouginot, J., Rignot, E., Bjørk, A. A., van den Broeke, M., Millan, R., Morlighem, M., ... Wood, M. (2019, May). Forty-six years of Greenland Ice Sheet mass balance from 1972 to 2018. *Proc. Natl. Acad. Sci.*, *116*, 9239–9244. doi: 10.1073/pnas.1904242116

Muntjewerf, L., Petrini, M., Vizcaino, M., Ernani da Silva, C., Sellevold, R., Scherrenberg, M. D. W., ... Lofverstrom, M. (2020). Greenland Ice Sheet Contribution to 21st Century Sea Level Rise as Simulated by the Coupled CESM2.1-CISM2.1. *Geophys. Res. Lett.*, *47*, e2019GL086836. doi: 10.1029/2019GL086836

Muntjewerf, L., Sacks, W. J., Lofverstrom, M., Fyke, J., Lipscomb, W. H., Ernani da Silva, C., ... Sellevold, R. (2021). Description and Demonstration of the Coupled Community Earth System Model v2 – Community Ice Sheet Model v2 (CESM2-CISM2). *J. Adv. Model. Earth Syst.*, *13*, e2020MS002356. doi: 10.1029/2020MS002356

Swingedouw, D., Rodehacke, C. B., Olsen, S. M., Menary, M., Gao, Y., Mikolajewicz, U., & Mignot, J. (2015, June). On the reduced sensitivity of the Atlantic overturning to Greenland ice sheet melting in projections: A multi-model assessment. *Clim. Dyn.*, *44*, 3261–3279. doi: 10.1007/s00382-014-2270-x

Todd, A., Zanna, L., Couldrey, M., Gregory, J., Wu, Q., Church, J. A., ... Zhang, X. (2020). Ocean-Only FAFMIP: Understanding Regional Patterns of Ocean Heat Content and Dynamic Sea Level Change. *J. Adv. Model. Earth Syst.*, *12*, e2019MS002027. doi: 10.1029/2019MS002027

| **Variable description** | **Units** | **CMIP6 name** |
|---|---|---|
| Eastward wind stress | [N/m$^2$] | taux |
| Northward wind stress | [N/m$^2$] | tauy |
| Sea ice concentration [a] | [0–1] | siconc |
| Near-surface temperature | [K] | tas |
| Near-surface humidity | [kg/kg] | huss |
| Downward shortwave radiation | [W/m$^2$] | rsds |
| Downward longwave radiation | [W/m$^2$] | rlds |
| Near-surface wind speed | [m/s] | sfcWind |
| Additional heat flux [b] | [W/m$^2$] | – |
| Restoring SSS under sea ice | [psu] | sos |
| Precipitation | [kg/m$^2$/s] | pr |
| Runoff [b] | [kg/m$^2$/s] | – |
| Additional FW flux [b] | [kg/m$^2$/s] | – |

[a] The forcing field that is passed to the model is sea surface temperatures (SST) instead of the actual sea ice concentrations. However, these SSTs are converted to sea ice concentrations via a linear relation in the model code and the SSTs are not used otherwise.

[b] Not modified

**Table S1.** Forcing variables of POP and their corresponding CMIP6 variables

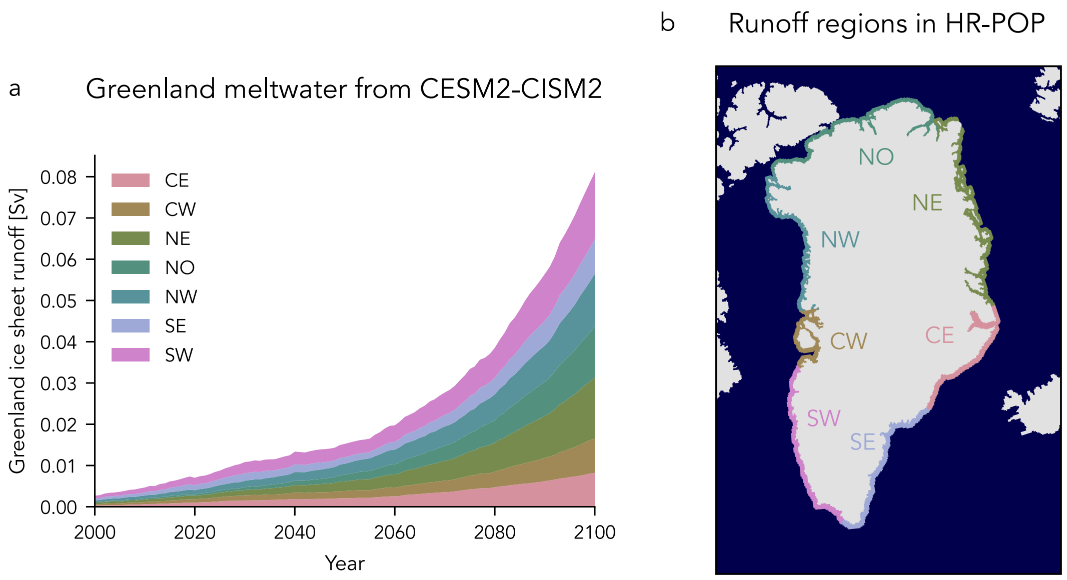


**Figure S1.** (a) Greenland meltwater input timeseries by region, (b) Regional distribution of Greenland meltwater into HR-POP.

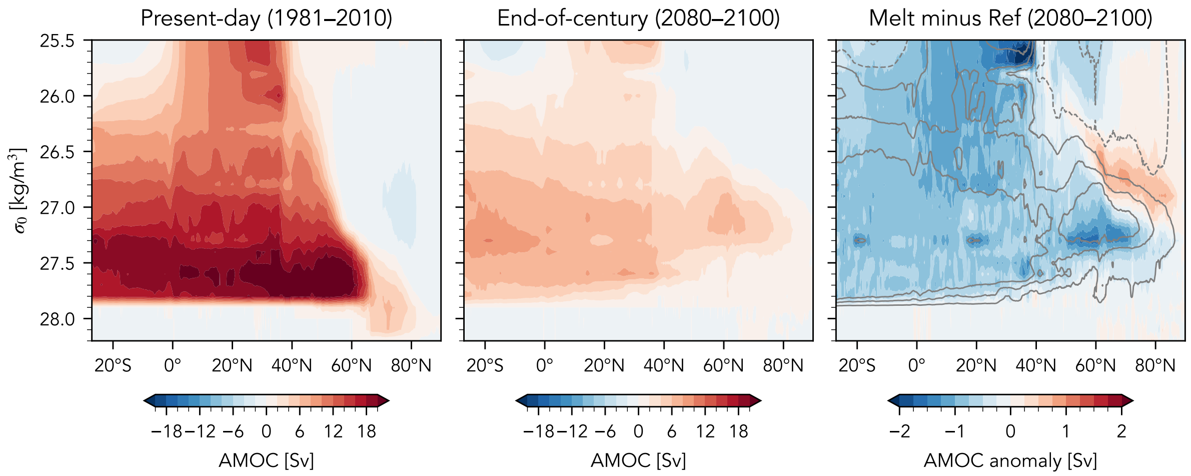


**Figure S2.** AMOC streamfunction in HR-POP in density coordinates referenced to the surface ($\sigma_0$). Climatologies of the "Reference" simulation for (a) the present-day (1981–2010) and (b) the end of the 21st century (2080–2100). The difference between the "Meltwater" and the "Reference" simulation at the end of the 21st century is shown in panel c.

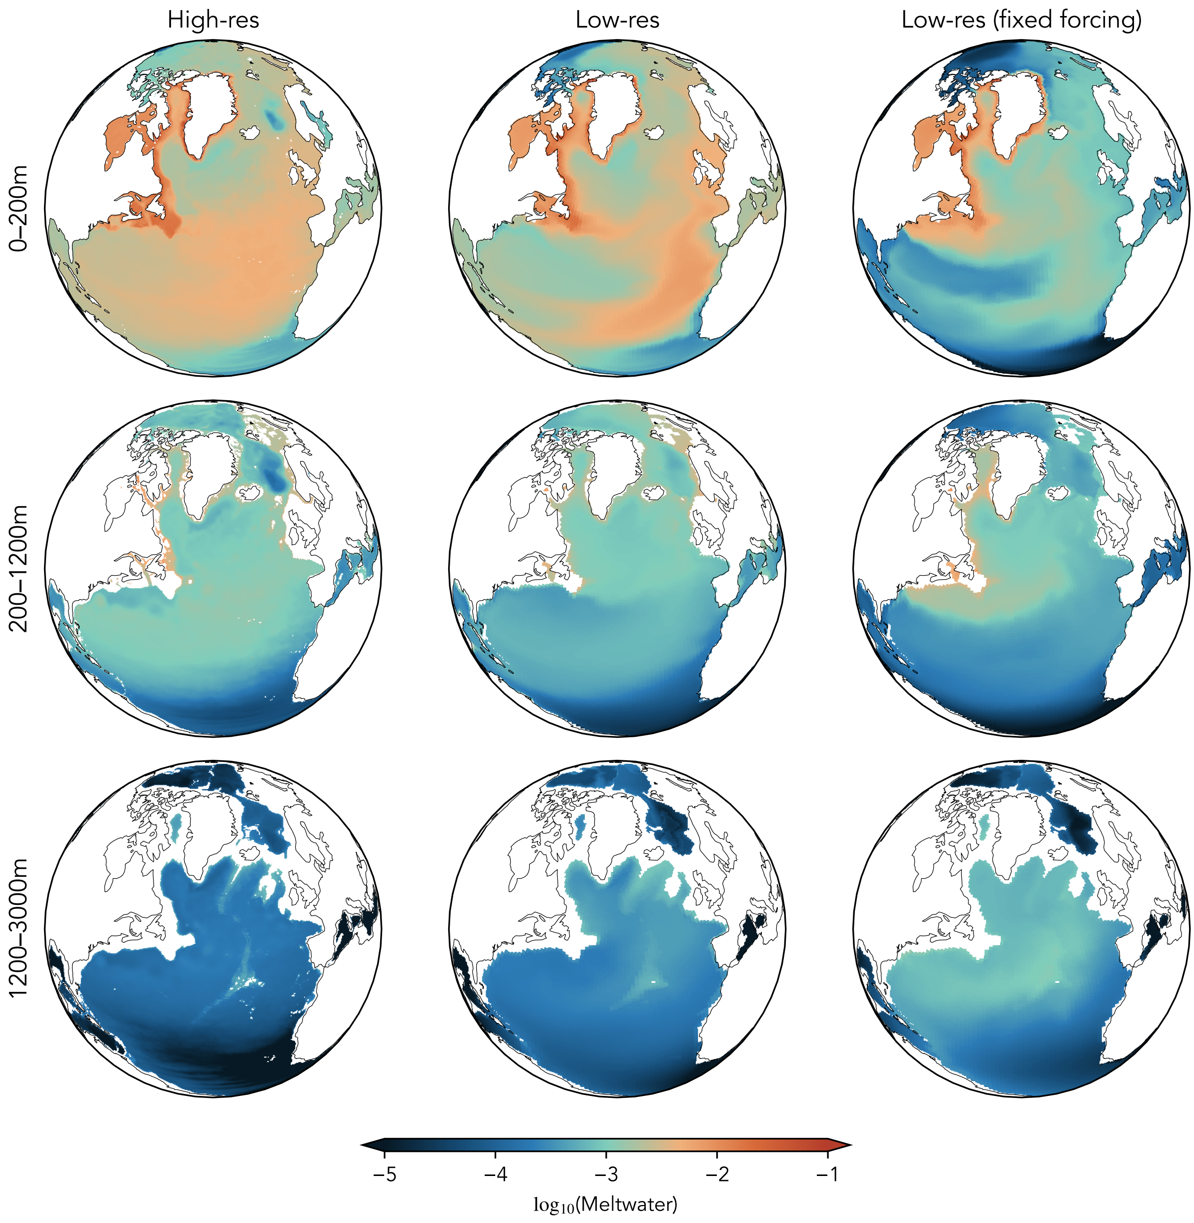


**Figure S3.** Vertically averaged concentration of the meltwater tracer (logarithmic scale) at three different depth levels: 0–200 m (first row), 200–1200 m (second row), 1200–3000 m (third row). The three columns represent HR-POP under SSP5-8.5 forcing, LR-POP under SSP5-8.5 forcing, and LR-POP under "normal-year" forcing with Greenland meltwater, respectively. All fields are averaged over 2080–2100.

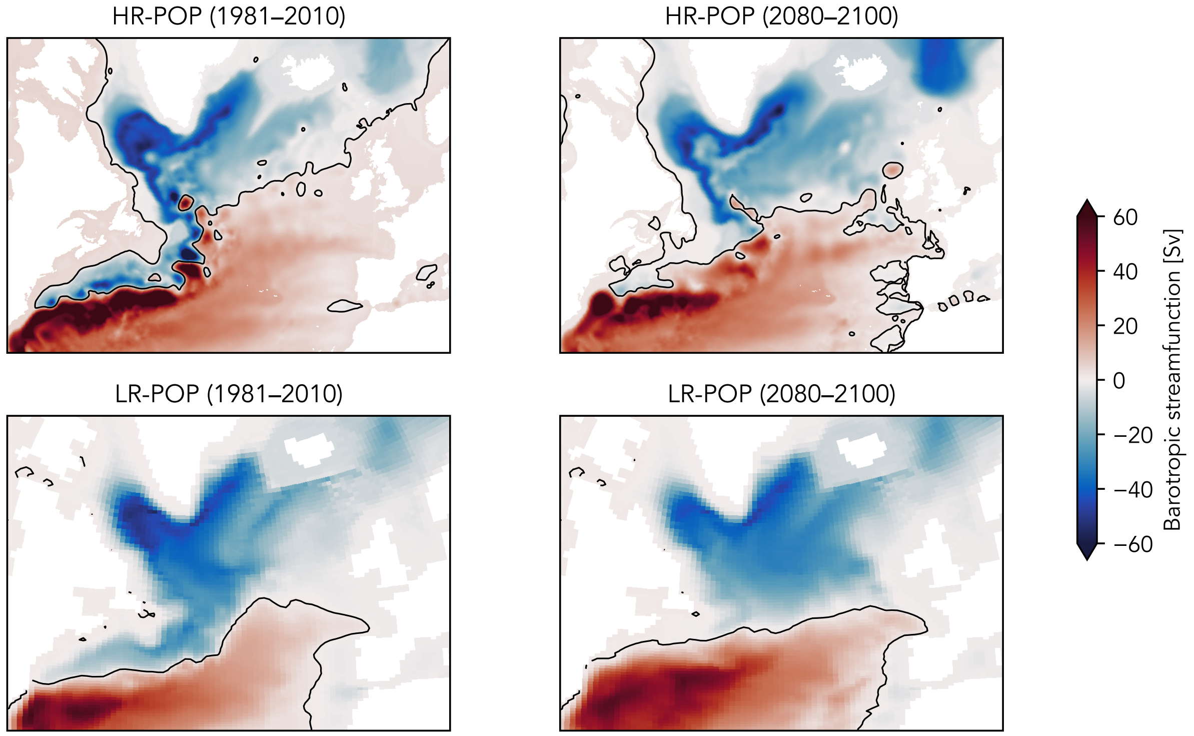


**Figure S4.** Annual mean barotropic streamfunction in the North Atlantic for HR-POP (first row) and LR-POP (second row) for 1981–2010 (first column) and 2080–2100 (second column). For 2080–2100, streamfunctions from the "Meltwater" simulations are shown, but they do not differ strongly from the "Reference" simulations for the same period. At both resolutions, the boundary between the subpolar and subtropical gyres (black line = zero contour) is much more zonal in the future period, consistent with Swingedouw et al. (2015).
